# Supplementary material for: Mechanical annealing and memories in a disordered solid
Source: arXiv:2112.07008 source file (2021-12-13)
Supplement: Supplementary file 1 [file SI-annealing.pdf]

# Supplementary Information for
# Mechanical annealing and memories in a disordered solid

Nathan C. Keim and Dani Medina

## SPATIOTEMPORAL STRUCTURE OF REARRANGEMENTS

Figure S1 explores the role of the $D^2_{\text{min}}$ threshold used to determine whether a particle has participated in a rearrangement. In the text and in past analyses [1, 2] this is 0.015. Doubling or halving the threshold shrinks or grows the spatial extents of soft spots in our results as compared to Figs. 5(c, d), but it does not qualitatively change the distribution of strain thresholds $\gamma_i^\pm$ as compared to Fig. 5e, so that these measurements remain consistent with each sample's response to amplitude variation (Fig. 4).

Figure S2 shows maps of $\gamma_i^\pm$ for Sample B, as Fig. 5(c, d) does for Sample A. Unlike in Sample A, a small number of particles did not return to the same positions at the end of the cycle; they are marked in green.

### Nonuniform shear strain

We find that particles near the middle of the material (i.e. halfway between the needle and the wall) systematically lag behind the displacements that would be expected for uniform shear. This is due to the weak coupling of the interfacial material to the bulk (oil and water) viscous flow, which has a different velocity profile [3, 4]. This lag is evident when comparing particle positions in two video frames that are ostensibly at the same value of global strain, but were taken during forward and reverse shear—as in the sampling protocol illustrated in Fig. 5a that was used to measure particles' $\gamma_i^\pm$.

To illustrate this effect, Fig. S3 compares particles' horizontal $x$ positions between forward and reverse shear, averaged over 10 pairs of frames in the analysis of sample "B" near $\gamma = 0$, when the strain rate and the lag are largest. We plot half the difference, $\Delta x/2$, as a function of position $y$ across the channel; the top of each image (near the fixed wall) is $y = 0$. Measurements are divided into 20 equally-spaced bins in $y$. Given the roughly uniform distribution of soft spots with respect to $y$, we would expect $\Delta x/2$ to average out to zero throughout the material, but instead there is a clear systematic difference, which is also evident in the image subtraction data described below. A positive $\Delta x/2$ means that a particle's $x$ is larger during forward shear ($\dot{\gamma} > 0$), so that it lags behind the needle's motion (in the $-x$ direction for forward shear).

Examining the slopes in Fig. S3, we see that in these observations taken when the effect is largest, the local shear strain leads the global shear strain by ~0.15% near the needle ($y \lesssim 500\ \mu$m), and lags by ~0.2% near the wall. This means that the values of $\gamma_i^\pm$ we report in Fig. 5 would be slightly different if they could be based on local shear strain at each soft spot. The net effect on our analysis of memory is small and subtle. The material's memory is defined in terms of global shear strain, and so in that sense, the $\gamma_i^\pm$ we measure are appropriate for this analysis and do not need to be corrected. Instead, the effect on our analysis comes from the fact that we drive the experiment at fixed frequency, and so decreasing $\gamma_0$ will lower the maximum strain rate and make the lag due to this viscous flow proportionally smaller—slightly and non-uniformly shifting the apparent $\gamma_i^\pm$ from the values we measured in the cycle with $\gamma_0 = 5\%$. However, even this is unlikely to affect our conclusions: the prominent differences between Samples A and B in Fig. 6g are robust to perturbing particles' $\gamma_i^\pm$ by $\sim \pm 0.2\%$.

Further studies are needed to systematically study the role of finite strain rate in this and other experiments. However, we note that the lagging effect we have discussed is an artifact of our experimental system's quasi-2D geometry [3], and not of the sampling and measurement methods we describe in the paper. In 3D materials, it should be possible to avoid this type of strain non-uniformity altogether.

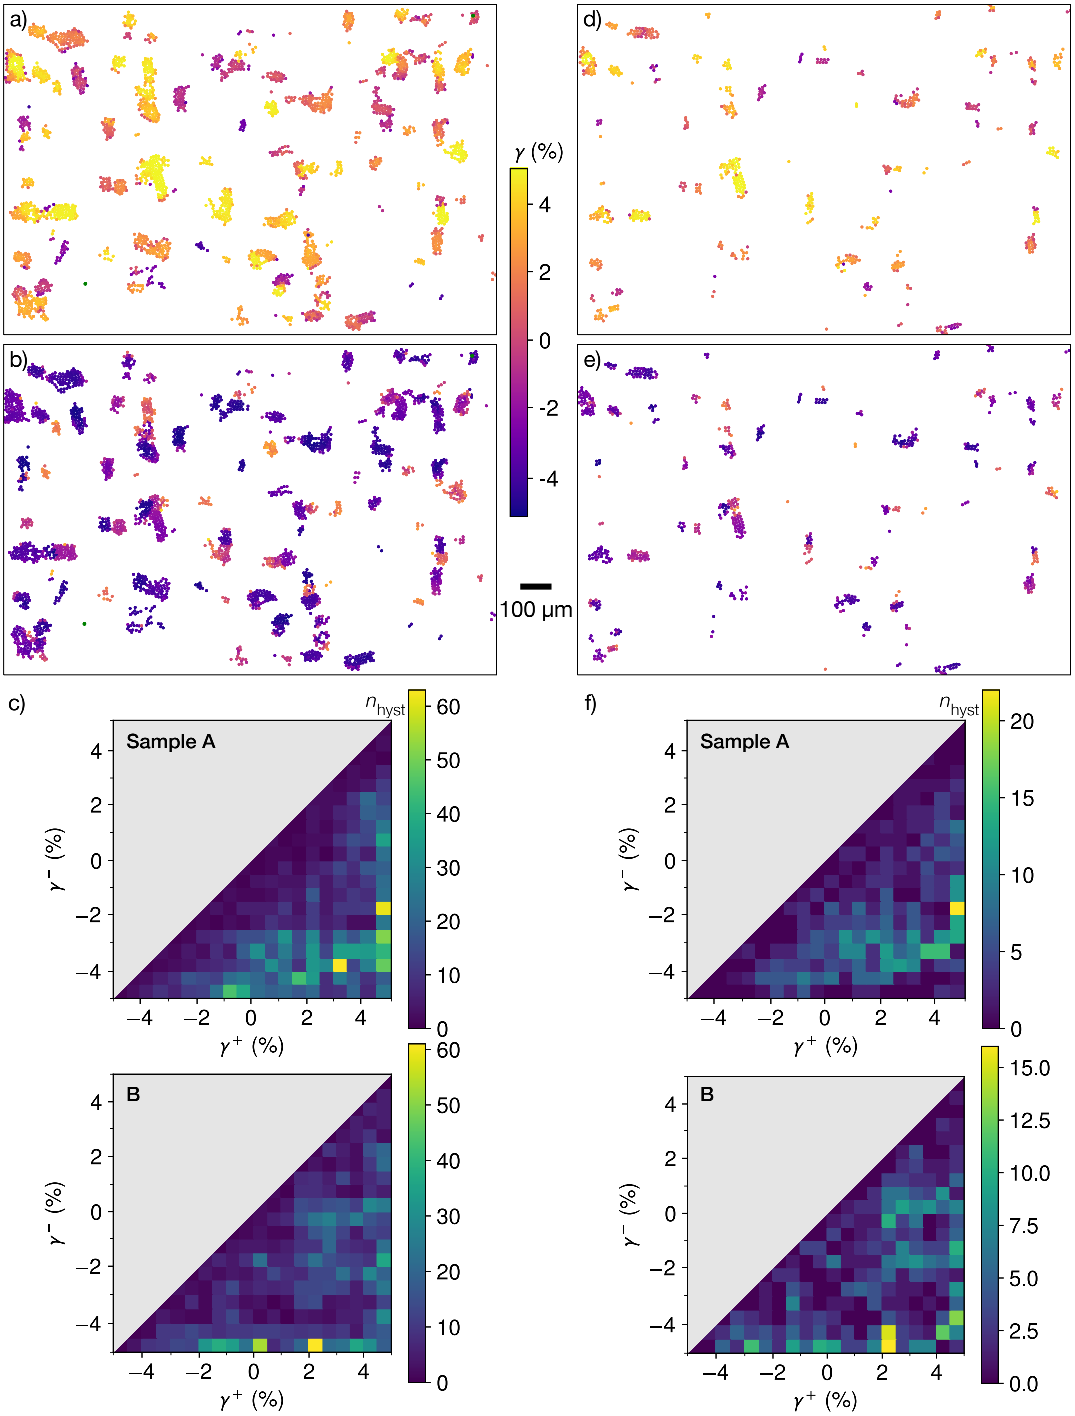


FIG. S1. Spatiotemporal structure of rearrangements as in Figs. 5(c, d, e), for alternate values of the $D^2_{\text{min}}$ threshold. Plots show particles colored by $\gamma_i^+$ and $\gamma_i^-$ for Sample A, and histograms of $\gamma_i^\pm$ for both samples. Analysis in the paper uses threshold 0.015, while **(a, b, c)** use the threshold 0.0075, and **(d, e, f)** use threshold 0.03.

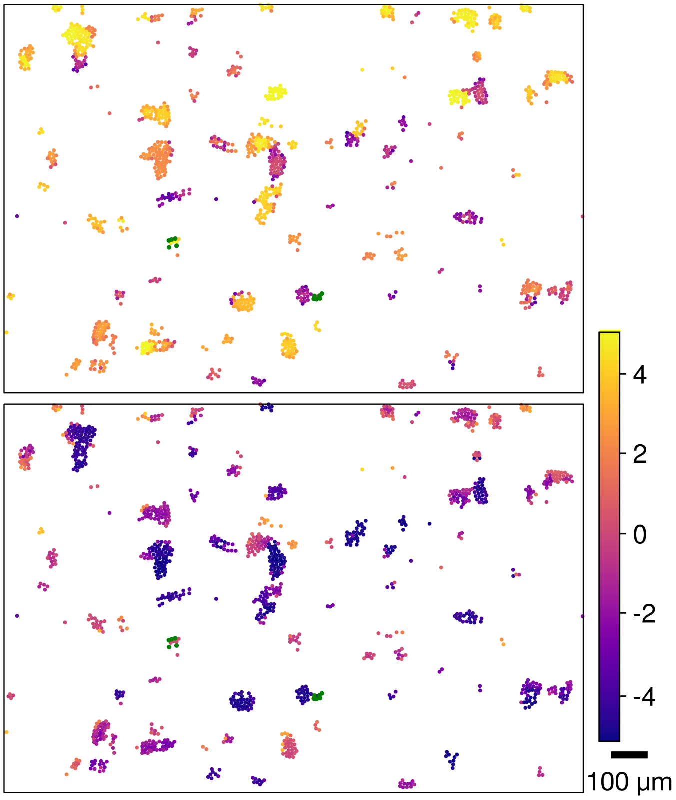


FIG. S2. Rearranging particles in Sample B, colored by $\gamma_i^+$ and $\gamma_i^-$, as the counterpart to the Sample A results in Figs. 5(c, d). In this case several rearranging particles were discarded because their trajectories were not closed; they are marked in green.

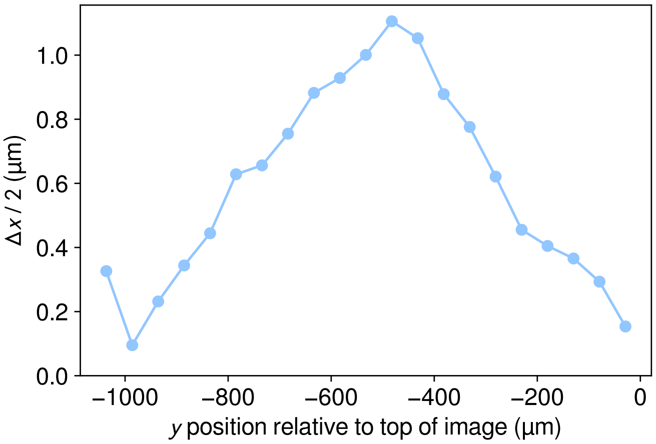


FIG. S3. Profile of lagging displacements. The horizontal $x$ positions of particles are compared between forward and reverse shear within a single cycle, in pairs of frames with matched values of strain $\gamma$. Particles are binned according to $y$ position, with $y = 0$ corresponding to the top of each video frame, near the fixed wall. 10 pairs of frames are averaged near $\gamma = 0$, when strain rate is fastest and the lag is largest. Plot shows the half-difference $\Delta x/2$. Uniform shear with no lag would correspond to $\Delta x = 0$; instead, particles lag behind the expected displacement, making the shear strain slightly nonuniform.

## SUPPORTING DATA FILES

A URL to a permanent, downloadable archive of supporting data is provided in the paper. It contains image data sufficient to verify all of the qualitative results in the paper, in 4 directories:

- `asymmetry` has the raw images corresponding to the beginning of each of the curves in Fig. 2c, as well as from 12 additional ring-down movies. The mean and standard deviation of the asymmetry ratio $b/c$ are reported in the text for these 13 frames taken from ring-down movies.
- `readout` has image subtractions from readout, corresponding to the MSD calculations for all readouts shown in Fig. 1e and Figs. 3(c, d).
- `nested` has image subtractions corresponding to all MSD calculations in Fig. 4b, for Samples A and B.
- `cycle` has image subtractions between each image during forward shear and its counterpart during reverse shear, corresponding to the $D^2_{\text{min}}$ calculations used to obtain $\gamma^+$ and $\gamma^-$ in Figs. 5(c, d) and Fig. S2, for samples A and B respectively. Files are labeled with the strain value of each pair.

### Static structure images

Figure S4 shows an example image of static structure from the `asymmetry` directory, from which $g(r, \theta)$ may be calculated as in the paper. The horizontally-moving needle is at the bottom of each image, a fixed wall is at the top, and the magnification is 0.665 $\mu$m/pixel. Some frames in `asymmetry` show small aggregates that formed gradually over the 23-hour run of experiments due to the weakening of repulsive forces, presumably from the presence of trace surfactants [5]. A smaller number of frames also have "voids"—regions 25–140 $\mu$m in size that are nearly devoid of particles, possibly due to a monolayer of adsorbed, insoluble contaminant.

### Subtracted images

The subtracted images show that our qualitative results can be reproduced with this simple method, instead of particle tracking. Figure S5 shows two examples from the data archive, representing the recovery of a memory during readout, and the rearrangements caused by exceeding the constant annealing amplitude. To produce these subtracted images from a pair of raw images, we convert each raw image to floating-point values between 0 and 1, subtract the earlier frame from the later one, and then clip the result to the range $[-0.5, 0.5]$ to make differences more visible; grey values in the resulting image files represent this range.

Soft spot rearrangements are apparent in images such as Fig. S5b as localized clusters of displaced particles, with an approximately quadrupolar morphology as in Fig. 1a [6, 7]. Some images also show large-scale perturbations from mechanical noise that affects the needle and camera positions, and small mismatches in strain due to the finite frame rate. These are all rejected by the quantitative methods used in the paper and described in its Materials and Methods section, which use the displacement of each particle relative to nearby particles. Taken together, these images also show that the aggregates and voids act as rigid inclusions and do not appear to play any special role in rearrangements or memory—for example, the two small voids in the material in Fig. S5 that are visible only because of a small global displacement.

The subtracted images in the `cycle` directory, based on the sampling protocol illustrated in Fig. 5a, deserve additional comment. Because we always subtract the earlier frame from the later one, the displacements switch signs near $\gamma = 0$, when we switch from making comparisons in the first half of the sampled cycle to the second half. Additionally, these images show the slight large-scale nonuniformity of the shear

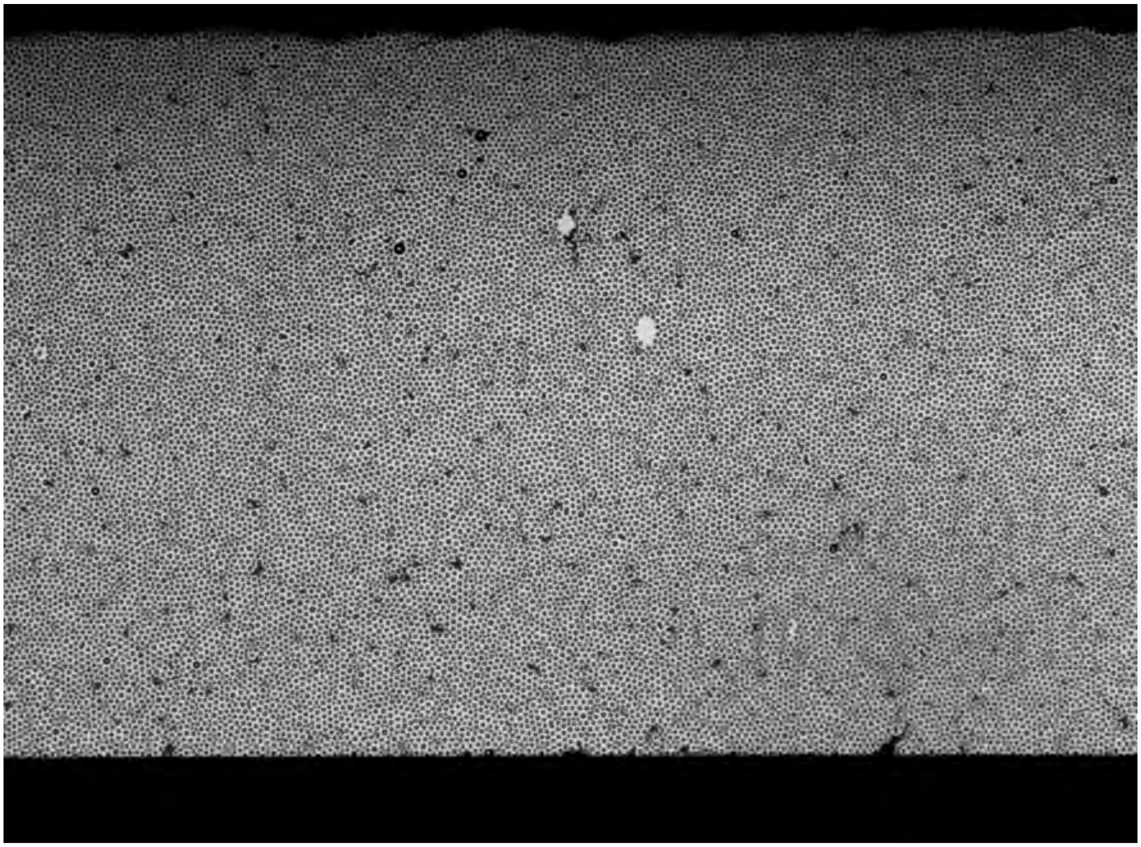

FIG. S4. Example raw image of static structure prepared by ring-down annealing. Width is 1550 $\mu$m. Fixed wall is at top; moving needle is at bottom. Sporadic small particle aggregates and two voids are visible.

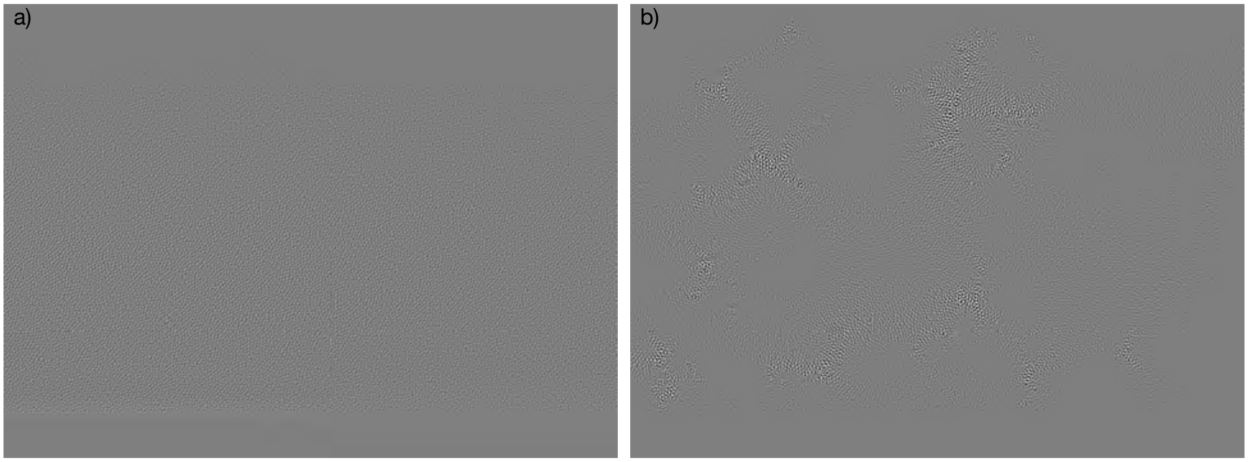


FIG. S5. Representative images from memory readout after constant-amplitude annealing at 4% and writing of a memory of 3% strain. **(a)** After a readout cycle with amplitude 3%, subtracting the image taken before readout reveals only small global displacements, indicating that the state before readout is recovered. **(b)** A readout cycle of amplitude 5% exceeds the annealing amplitude, resulting in several large new rearrangements. Width of each image is 1550 $\mu$m.

deformation discussed above, and confirm that the effect disappears as the needle slows down near the extrema of strain.

---

[1] Nathan C Keim and Paulo E Arratia, "Mechanical and microscopic properties of the reversible plastic regime in a 2d jammed material," Phys. Rev. Lett. **112**, 028302 (2014).

[2] Nathan C Keim and Paulo E Arratia, "Role of disorder in finite-amplitude shear of a 2d jammed material," Soft Matter **11**, 1539–1546 (2015).

[3] Sven Reynaert, Carlton F Brooks, Paula Moldenaers, Jan Vermant, and Gerald G Fuller, "Analysis of the magnetic rod interfacial stress rheometer," Journal of Rheology **52**, 261–285 (2008).

[4] Tom Verwijlen, Paula Moldenaers, Howard A Stone, and Jan Vermant, "Study of the flow field in the magnetic rod interfacial stress rheometer," Langmuir **27**, 9345–9358 (2011).

[5] Bum Jun Park, John P Pantina, Eric M Furst, Martin Oettel, Sven Reynaert, and Jan Vermant, "Direct measurements of the effects of salt and surfactant on interaction forces between colloidal particles at water-oil interfaces," Langmuir **24**, 1686–1694 (2008).

[6] J D Eshelby, "The determination of the elastic field of an ellipsoidal inclusion, and related problems," Proceedings of the Royal Society of London A: Mathematical, Physical and Engineering Sciences **241**, 376–396 (1957).

[7] G Picard, A Ajdari, F Lequeux, and Lydéric Bocquet, "Elastic consequences of a single plastic event: A step towards the microscopic modeling of the flow of yield stress fluids," The European Physical Journal E **15**, 371–381 (2004).
